# Supplementary material for: Deep Reactive Planning in Dynamic Environments
Source: arXiv:2011.00155 source file (2020-11-05)
Supplement: Supplementary file 1 [file appendix.tex]

\clearpage

\input{exp_sim2real_cyclegan}

\input{exp_sim2real_waypoints_no_obs}

\clearpage
\input{exp_insertion}
\clearpage
